# Supplementary material for: Collective stiffening of soft hair assemblies
Source: arXiv:2002.02834 source file (2020-05-22)
Supplement: Supplementary file 1 [file SupplementalMaterial.pdf]

# Supplemental Material for:
# *Collective stiffening of soft hair assemblies*

J.-B. Thomazo, E. Lauga, B. Le Révérend, E. Wandersman and A. M. Prevost

February 7, 2020

## 1 Materials and methods

### 1.1 Imaging

Imaging of the pillars summits were performed with a 5× microscope air objective (Plan–Apo, Edmunds Optics, USA), in combination with a fast and sensitive camera (BlackFly S, 2448×2048 pixels$^2$, 12 bits, 75 frames/s (fps) at full frame, Flir, USA), a dichroic filter and an emission filter (MD498 and MF525-39 respectively, Thorlabs, USA). Illumination was provided by a high power blue LED ($\lambda = 465 \pm 5$ nm, Sodial(r)). With the chosen 5× magnification, images have a spatial resolution of 0.7 $\mu$m per pixel. Rheometer data and images were acquired simultaneously using a TTL trigger signal sent by the rheometer (controlled by its dedicated software Rheocompass 1.19, Anton Paar) to the camera, once rotation of the upper plate initiates.

### 1.2 Soft hair assembly fabrication

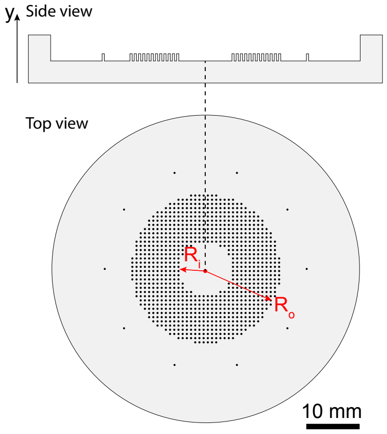


Figure 1: Sketch of the soft hair assembly pool. (a) Side view along a diameter. The vertical axis is noted $y$. (b) Top view of the bottom of the pool. Two patterns have been designed, a dense one and a sparse one.

Molds were obtained by microdrilling a Plexiglas substrate with microdrills of diameter $2a = 100$ $\mu$m (Performance Micro Tool, USA) using a CNC desktop milling machine (Minitech, USA). Ten equally spaced holes were drilled on a circle of radius 15 mm to obtain the reference pattern (with a number density of 0.04 mm$^{-2}$. Densely distributed holes were drilled on a square lattice of mesh size $d$ and number density $n$ ranging from 1 to 10 holes per mm$^2$, on an annulus whose constant outer diameter is $R_o = 10$ mm and whose inner diameter $R_i = R_o - 10d$ (Fig. 1). For all holes, their depth was set to 450 $\mu$m. Fluorescent particles (diameter [1–5] $\mu$m, GFM, Cospheric, 1.3g/cc) were first deposited at the bottom of the microholes using the same protocol as described in [1].

As in [1], soft hair assemblies were obtained by pouring in the molds a liquid PDMS (PolyDimethylSiloxane, Sylgard 184, Dow Corning, USA) melt – crosslinker mixture in a 10:1 stoichiometric ratio, followed by a curing in an oven (12 hours, $T = 65$°C) and eventually an unmolding. Note that abrupt unmolding of the substrate could induce occasional tearing of some of the pillars as clearly evidenced for three pillars on the right half of the image of Fig. 1b in the main text. We found that injecting isopropanol at the Plexiglas–elastomer interface

prior to unmolding minimized such tearing. Measurements of the pillars length $L$ were performed using optical microscopy, yielding an actual $L = 435 \pm 7$ $\mu$m.

### 1.3 Preparation and characterization of solutions

Solutions of glycerol (Sigma-Aldrich) mixed in Millipore deionized water at different concentration were used. Their dynamic viscosities $\eta$ were measured with the rheometer operating in a plate-plate geometry with a 1 mm gap and a shear rate $\dot{\gamma}$ varying from 1 to 100 s$^{-1}$. To obtain the data of Fig. 3a in the main text, three mixing glycerol/water mixing ratios were actually used. For most of the data, a 95 % w/wt glycerol/water ratio was used, yielding a dynamic viscosity $\eta = 0.42 \pm 0.08$ Pa.s at room temperature. To further check that the results of Fig. 3a do not depend on the viscosity of the solution, two additional viscosities of $\approx 0.1$ Pa.s and $\approx 0.8$ Pa.s respectively were also used.

## 2 Lattice topology dependence of the microscopic model

Using the microscopic model, we derived an expression for the ratio $\delta_q/\delta_0$ where $\delta$ stands for the deflection of a pillar $q$ in the presence of neighboring pillars and where

$$\delta_0 = K_0 \frac{\eta\dot{\gamma}L^5}{Ea^4} \tag{1}$$

is the deflection of an isolated pillar. Let us recall that this equation (Eq. 6 in the main text) is given by

$$\frac{\delta_q}{\delta_0} = \left| \mathbf{e}_x - L^3 \sum_{p\neq q} \frac{1}{|\mathbf{r}_{pq}|^3} (\mathbf{e}_x \cdot \mathbf{e}_{pq})\mathbf{e}_{pq} \right|, \tag{2}$$

where $\mathbf{e}_x$ stands for a unit vector in the direction of the flow, $\mathbf{r}_{pq}$ is the vector that joins pillars $p$ and $q$, and $\mathbf{e}_{pq} = \mathbf{r}_{pq}/|\mathbf{r}_{pq}|$ is a unit vector along $\mathbf{r}_{pq}$ (*see* Fig. 3b in the main text).

Here, we compute analytically the right-hand side of Eq. 2 for two distinct spatial distributions of pillars: a *square* lattice, like the one used in our experiments and a *hexagonal* one. In both cases, we show that $\delta/\delta_0$ does not depend on the orientation of the lattice with respect to the flow direction, where for sake of simplicity we have renamed $\delta_q$ by $\delta$. Since we expect flow perturbations to be much larger in the direction of the flow than in the transverse one, we thus only consider longitudinal flow perturbations along the $\mathbf{e}_x$ direction.

### 2.1 Case 1 – Square lattice

Let us first consider the square lattice of mesh size $d$ sketched in Fig 2. Positions of the pillars $p$, noted $r_{ij}$, are identified with their coordinates $i$ and $j$ in the $(\mathbf{e}_i, \mathbf{e}_j)$ unit vector basis. One therefore has $\mathbf{r}_{ij} = d\,(i\mathbf{e}_i + j\mathbf{e}_j)$. Defining $\mathbf{e}_{ij} = \mathbf{r}_{ij}/|\mathbf{r}_{ij}|$ and keeping only the projected components along $\mathbf{e}_x$, Eq. 2 become

$$\frac{\delta}{\delta_0} = 1 - \frac{L^3}{d^3} \sum_{i^2+j^2\neq 0} S_{ij} \quad \text{where} \quad S_{ij} = \frac{(\mathbf{e}_x \cdot \mathbf{e}_{ij})^2}{(i^2+j^2)^{3/2}}. \tag{3}$$

For a lattice tilted by an angle $\theta$ with respect to the direction of the flow $\mathbf{e}_x$, one has

$$\begin{aligned} \mathbf{e}_i &= \cos\theta\ \mathbf{e}_x - \sin\theta\ \mathbf{e}_z, \\ \mathbf{e}_j &= \sin\theta\ \mathbf{e}_x + \cos\theta\ \mathbf{e}_z, \end{aligned} \tag{4}$$

with $\mathbf{e}_z$ a unit vector in the direction transverse to the flow. One thus obtains that

$$\mathbf{e}_x \cdot \mathbf{e}_{ij} = \frac{i\cos\theta + j\sin\theta}{\sqrt{i^2+j^2}} \quad \text{and} \quad S_{ij} = \frac{(i\cos\theta + j\sin\theta)^2}{(i^2+j^2)^{5/2}}. \tag{5}$$

Equation 3 can then be rewritten as

$$\frac{\delta}{\delta_0} = 1 - S\frac{L^3}{d^3} = 1 - S\left(\frac{n}{n_0}\right)^{3/2} \quad \text{where} \quad S = \sum_{i^2+j^2\neq 0} S_{ij}, \tag{6}$$

and where $n = 1/d^2$ is the number density of pillars and $n_0 = 1/L^2$.

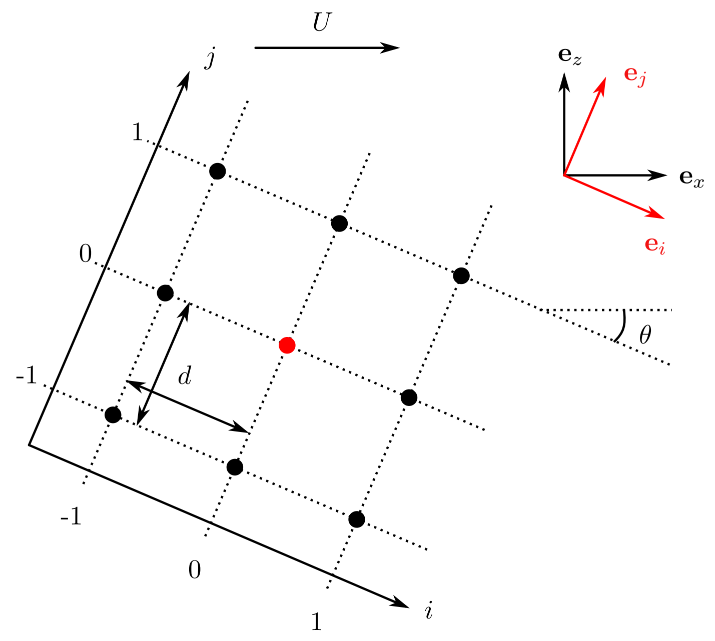


Figure 2: Sketch of a tilted square lattice of pillars of mesh size $d$ (top view). The flow has speed $U$ along the $x$ direction. The lattice is tilted by an angle $\theta$ with respect to $U$. Pillars are located with their coordinates $i$ and $j$.

One is now left with the computation of the parameter $S$. For this, on can decompose it as the sum of 4 terms as

$$\begin{aligned} S &= \sum_{i^2+j^2\neq 0} S_{ij} \\ &= \sum_{i\in\mathbb{Z}^*} S_{i0} + \sum_{j\in\mathbb{Z}^*} S_{0j} + \sum_{i>0}\sum_{j\in\mathbb{Z}^*} S_{ij} + \sum_{i<0}\sum_{j\in\mathbb{Z}^*} S_{ij} \\ &= S_{j=0} + S_{i=0} + S_{i>0} + S_{i<0}. \end{aligned} \tag{7}$$

The calculation of the first two terms gives

$$S_{j=0} = \sum_{i\in\mathbb{Z}^*} S_{i0} = \sum_{i\in\mathbb{Z}^*} \frac{\cos^2\theta}{|i|^3} = 2\sum_{i=1}^{\infty}\frac{\cos^2\theta}{i^3}, \tag{8}$$

$$S_{i=0} = \sum_{j\in\mathbb{Z}^*} S_{0j} = \sum_{j\in\mathbb{Z}^*} \frac{\sin^2\theta}{|j|^3} = 2\sum_{j=1}^{\infty}\frac{\sin^2\theta}{j^3}. \tag{9}$$

Hence

$$S_{j=0} + S_{i=0} = 2\sum_{i=1}^{\infty}\frac{1}{i^3}. \tag{10}$$

The term $S_{i>0}$ can also be decomposed as follows

$$\begin{aligned} S_{i>0} &= \sum_{i>0}\sum_{j\in\mathbb{Z}^*} S_{ij} \\ &= \sum_{i>0}\left[\sum_{j<0} S_{ij} + \sum_{j>0} S_{ij}\right] \\ &= \sum_{i>0}\sum_{j>0}\left[S_{ij} + S_{i-j}\right] \\ &= \sum_{i>0}\sum_{j>0}\left[\frac{(i\cos\theta + j\sin\theta)^2}{(i^2+j^2)^{5/2}} + \frac{(i\cos\theta - j\sin\theta)^2}{(i^2+j^2)^{5/2}}\right] \\ &= 2\sum_{i>0}\sum_{j>0}\frac{i^2\cos^2\theta + j^2\sin^2\theta}{(i^2+j^2)^{5/2}}. \end{aligned} \tag{11}$$

On can note that for each couple $(i,j)$, there is a corresponding couple $(j,i)$, which implies that Eq. 11 can be rewritten as follows

$$\begin{aligned} S_{i>0} &= \sum_{i>0}\sum_{j>0}\left[\frac{i^2\cos^2\theta + j^2\sin^2\theta}{(i^2+j^2)^{5/2}} + \frac{j^2\cos^2\theta + i^2\sin^2\theta}{(j^2+i^2)^{5/2}}\right] \\ &= \sum_{i>0}\sum_{j>0}\frac{i^2+j^2}{(i^2+j^2)^{5/2}} \\ &= \sum_{i>0}\sum_{j>0}\frac{1}{(i^2+j^2)^{3/2}}. \end{aligned} \tag{12}$$

In addition, for any $i$ or $j$ $S_{i>0} = S_{i<0}$. Consequently, one has

$$S = 2\left[\sum_{i,j=1}^{\infty}\frac{1}{(i^2+j^2)^{3/2}} + \sum_{i=1}^{\infty}\frac{1}{i^3}\right] = 2\sum_{i=0}^{\infty}\sum_{j=1}^{\infty}\frac{1}{(i^2+j^2)^{3/2}}. \tag{13}$$

Clearly, for a square lattice of pillars, $S$ and therefore $\delta/\delta_0$ (*see* Eq. 6) do not depend on the orientation $\theta$ of the lattice with respect to the flow direction. The value of $S$ has been evaluated with Mathematica 11 (Wolfram Research, Inc.) yielding $S \approx 4.51$. When limiting this evaluation to the first 5 nearest neighbors, *i.e* with $i$ and $j$ ranging from 0 to 5 and 1 to 5 respectively, like in our experiments, $S \approx 4$, *i.e* about 90% of its maximum value.

## 2.2 Case 2 – Hexagonal lattice

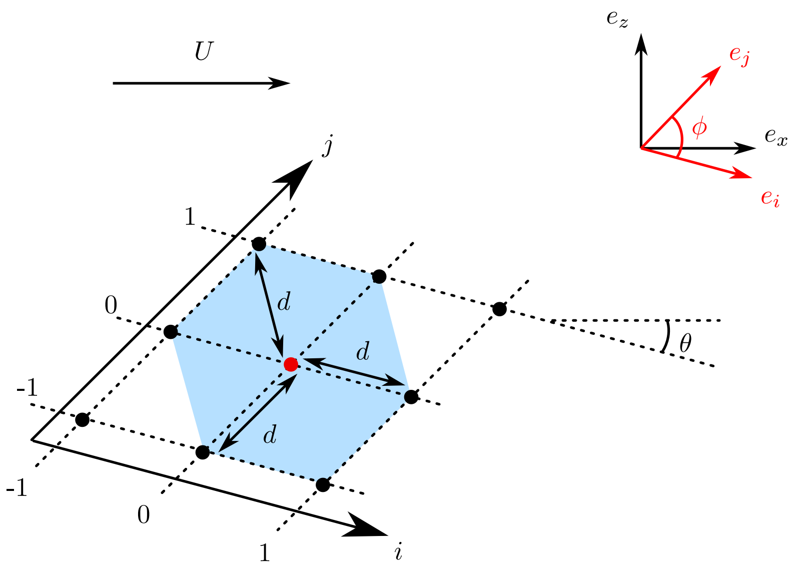


Figure 3: Sketch of a tilted hexagonal lattice of pillars of mesh size $d$ (top view). The lattice is tilted by an angle $\theta$ with respect to the direction of the flow along $\mathbf{e}_x$. Pillars are located with their coordinates $i$ and $j$ in the non-orthogonal basis of unit vectors $\mathbf{e}_i$ and $\mathbf{e}_j$ that form the angle $\phi = \pi/3$.

In the case of a hexagonal lattice, Eq. 2 can also be computed analytically. Again, let us consider the sketch of Fig. 3 that shows a top view of a hexagonal lattice of pillars tilted with an angle $\theta$ with respect to the direction of the flow $\mathbf{e}_x$. Positions of the pillars are given by their coordinates $(i,j)$ in the unit vectors basis $(\mathbf{e}_i, \mathbf{e}_j)$. In contrast to the square case, $\mathbf{e}_i$ and $\mathbf{e}_j$ are not orthogonal vectors and form an angle $\phi = \pi/3$ between them. $\theta$ being the angle between $\mathbf{e}_i$ and $\mathbf{e}_x$, one now has the following relations

$$\begin{aligned} \mathbf{e}_i &= \cos\theta\ \mathbf{e}_x - \sin\theta\ \mathbf{e}_z, \\ \mathbf{e}_j &= \cos(\theta-\phi)\ \mathbf{e}_x - \sin(\theta-\phi)\ \mathbf{e}_z. \end{aligned} \tag{14}$$

This time, the dot product $\mathbf{e}_i \cdot \mathbf{e}_j$ is not equal to zero and is given by

$$\mathbf{e}_i \cdot \mathbf{e}_j = \cos\theta\cos(\theta-\phi) + \sin\theta\sin(\theta-\phi) = \cos(\phi) = 1/2. \tag{15}$$

In the case of a hexagonal lattice, Eq. 2 projected onto the $x$–axis is the same as given by Eq. 3, albeit a modified expression for $S_{ij}$. Indeed, recalling that $\mathbf{e}_{ij} = \mathbf{r}_{ij}/|\mathbf{r}_{ij}|$, $\mathbf{r}_{ij} = d\,(i\mathbf{e}_i + j\mathbf{e}_j)$ and using Eq. 14, the dot product $\mathbf{e}_x \cdot \mathbf{e}_{ij}$ in Eq. 3 now equals

$$\mathbf{e}_x \cdot \mathbf{e}_{ij} = \frac{i\cos\theta + j\cos(\theta-\phi)}{|i\mathbf{e}_i + j\mathbf{e}_j|^3}. \tag{16}$$

Since

$$\begin{aligned} |i\mathbf{e}_i + j\mathbf{e}_j| &= \sqrt{(i\mathbf{e}_i + j\mathbf{e}_j)^2} \\ &= \sqrt{i^2 + 2ij\mathbf{e}_i \cdot \mathbf{e}_j + j^2} \\ &= \sqrt{i^2 + ij + j^2} \end{aligned} \tag{17}$$

one thus has

$$S_{ij} = \frac{(i\cos\theta + j\cos(\theta-\phi))^2}{(i^2+ij+j^2)^{5/2}} \tag{18}$$

We are now left to evaluating the parameter $S$ which is the discrete sum of all $S_{ij}$ terms with $(i,j) \in \mathbb{Z}^{*2}$ (*see* Eq. 3).

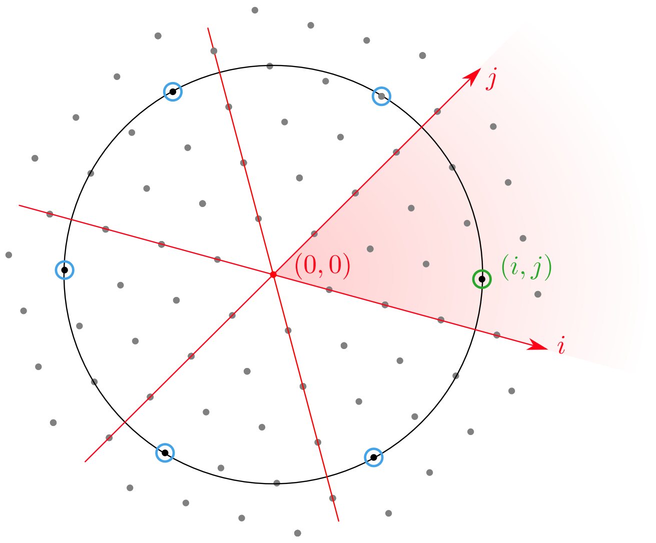


Figure 4: Sketch of a hexagonal lattice of pillars and principle of decomposition of $S$ (*see* main text for details).

Like in the square lattice case, the idea is to decompose $S$ as the sum of 6 distinct terms by taking advantage of the 6-fold symmetry of the hexagonal lattice. These terms can be obtained in the following way. First, let us consider Fig. 4 in which a portion of a hexagonal lattice of points has been sketched. By symmetry, the plane that contains all lattice points can be divided into 6 equal angular sectors bounded by the three red solid lines that intersect at point $(0,0)$. Next, consider a given point of coordinates $(i,j)$ (green circled point in Fig. 4) that belongs to one of those sectors, shaded in red in Fig. 4. In each other sector, there exists one and only one point of the hexagonal lattice whose distance from the origin $(0,0)$ is equal to $r_{ij}$ (blue circled points in Fig. 4 that lie on the circle of radius $r_{ij}$). The coordinates of these points in the $(\mathbf{e}_i, \mathbf{e}_j)$ basis can be found and expressed as function of $i$ and $j$ by simply applying successive rotations of angle $\phi = \pi/3$ to the vector $\mathbf{r}_{ij} = d \times (i\mathbf{e}_i + j\mathbf{e}_j)$ of the first initial point. This can be done graphically. After a first rotation, one finds for instance that the unit vectors $\mathbf{e}_i$ and $\mathbf{e}_j$ do transform into $\mathbf{e}_j$ and $-\mathbf{e}_i + \mathbf{e}_j$ respectively, which yields $(-j, i+j)$ as coordinates of the second point. Table 1 lists all found pairs of rotated unit vectors and $\mathbf{r}_{ij}$ coordinates (in $d$ units) of all 6 points after $n$ $(= 0$ to $5)$ rotations.

Knowing the coordinates of all 6 points in terms of the $(i,j)$ coordinates of the initial point then allows to rewrite the double sum in $S$ as

$$S = \sum_{i=0}^{\infty}\sum_{j=1}^{\infty}\left[S_{i,j} + S_{-j,i+j} + S_{-i-j,i} + S_{-i,-j} + S_{j,-i-j} + S_{i+j,-i}\right]. \tag{19}$$

| $n$ | 0 | 1 | 2 | 3 | 4 | 5 |
|---|---|---|---|---|---|---|
| Vector 1 | $\mathbf{e}_i$ | $\mathbf{e}_j$ | $-\mathbf{e}_i+\mathbf{e}_j$ | $-\mathbf{e}_i$ | $-\mathbf{e}_j$ | $\mathbf{e}_i-\mathbf{e}_j$ |
| Vector 2 | $\mathbf{e}_j$ | $-\mathbf{e}_i+\mathbf{e}_j$ | $-\mathbf{e}_i$ | $-\mathbf{e}_j$ | $\mathbf{e}_i-\mathbf{e}_j$ | $\mathbf{e}_i$ |
| $[\mathbf{M}_\phi^n \cdot \mathbf{r}_{ij}] \cdot \mathbf{e}_i$ | $i$ | $-j$ | $-i-j$ | $-i$ | $j$ | $i+j$ |
| $[\mathbf{M}_\phi^n \cdot \mathbf{r}_{ij}] \cdot \mathbf{e}_j$ | $j$ | $i+j$ | $i$ | $-j$ | $-i-j$ | $-i$ |

Table 1: Rotated unit vectors after $n$ rotations and deduced coordinates in the $(\mathbf{e}_i, \mathbf{e}_j)$ basis of the rotated $\mathbf{M}_\phi^n \cdot \mathbf{r}_{ij}$ vectors where $\mathbf{M}_\phi$ is the rotation matrix of angle $\phi$.

Since $S_{i,j} = S_{-i,-j}$, $S$ can be simplified further as

$$S = 2\sum_{i=0}^{\infty}\sum_{j=1}^{\infty} S_{i,j} + S_{-j,i+j} + S_{-i-j,i}. \tag{20}$$

In addition, since $r_{i,j} = r_{-j,i+j} = r_{-i-j,i}$, one is left to evaluating the following sum, denoted by $\varsigma$, only. Using the expression computed earlier for $S_{ij}$ and given by Eq. 18, one has

$$\begin{aligned}
\varsigma &= S_{i,j} + S_{-j,i+j} + S_{-i-j,i} \\
&= 1/r_{i,j}^3\,[(\mathbf{e}_x \cdot \mathbf{e}_{i,j})^2 + (\mathbf{e}_x \cdot \mathbf{e}_{-j,i+j})^2 + (\mathbf{e}_x \cdot \mathbf{e}_{-i-j,i})^2] \\
&= 1/r_{i,j}^5\,[(i\cos\theta + j\cos(\theta-\phi))^2 \\
&\qquad +(-j\cos\theta + (i+j)\cos(\theta-\phi))^2 \\
&\qquad +((-i-j)\cos\theta + i\cos(\theta-\phi))^2] \\
&= 1/r_{i,j}^5\,[(i^2+j^2+(-i-j)^2)\cos^2\theta \\
&\qquad +(2ij - 2j(i+j) + 2(-i-j)i)\cos\theta\cos(\theta-\phi) \\
&\qquad +(j^2+(i+j)^2+i^2)\cos^2(\theta-\phi)] \\
&= 2(i^2+ij+j^2)/r_{i,j}^5\,[\cos^2\theta - \cos\theta\cos(\theta-\phi) + \cos^2(\theta-\phi)] \\
&= 2/r_{i,j}^3\,[\cos^2\theta - \cos\theta\cos(\theta-\phi) + \cos^2(\theta-\phi)] \\
&= 2/r_{i,j}^3\,[\cos^2\theta - \frac{1}{2}\cos^2\theta - \frac{\sqrt{3}}{2}\sin\theta\cos\theta + \frac{3}{4}\sin^2\theta \\
&\qquad +\frac{\sqrt{3}}{2}\sin\theta\cos\theta + \frac{1}{4}\cos^2\theta] \\
&= \frac{3}{2(i^2+ij+j^2)^{3/2}}.
\end{aligned}$$

In the end, $S$ can thus be simplified to the following expression

$$S = 3\sum_{i=0}^{\infty}\sum_{j=1}^{\infty} \frac{1}{(i^2+ij+j^2)^{3/2}}. \tag{21}$$

Like in the case of a square lattice case, the value of $S$, and therefore thst of $\delta/\delta_0$ (*see* Eq. 6), do not depend on the orientation $\theta$ of the lattice with respect to the flow direction. $S$ has been evaluated with Mathematica 11 (Wolfram Research, Inc.) yielding $S \approx 5.51$.

# 3 Bibliography

[1] J.-B. Thomazo, J. Contreras Pastenes, C. J. Pipe, B. Le Révérend, E. Wandersman, and A. M. Prevost, Journal of the Royal Society Interface **16**, 20190362 (2019).
